# Supplementary material for: ES-KT-24: A Multimodal Knowledge Tracing Benchmark Dataset with Educational Game Playing Video and Synthetic Text Generation
Source: arXiv:2409.10244 source file (2024-09-16)
Supplement: Supplementary file 1 [file 8_appendix.tex]

\appendix

\section{Appendix}
\label{sec:appendix}

This is an appendix.
